# Supplementary material for: Revealing Decurve Flows for Generalized Graph Propagation
Source: arXiv:2402.08480 source file (2024-02-13)
Supplement: Supplementary file 1 [file curvature.tex]

\clearpage
\section{Appendix}

\subsection{Casting Prior Methods to Generalised Propagation Framework}

\subsection{Ricci curvature on weighted directed graphs}
\begin{definition}
\textcolor{red}{(Weighted Directed Graph)} A \textit{weighted directed graph} $G=(V, w)$ is a directed graph $G=(V, E)$ equipped with a function $w: V \times V \rightarrow[0, \infty)$, where $w(x, y)>0$ if and only if $(x, y) \in E$, denoted as $x \rightarrow y$. The function $w$ is called the \textit{edge weights} and we denote $w(x, y)$ as $w_{xy}$ for convenience.
\end{definition}

\begin{definition}
\textcolor{red}{(Strongly Connected)} In a directed graph, two vertices $u$ and $v$ are strongly connected if there exists a directed path from $x$ to $y$, then there exists a directed path from $y$ to $x$. A weighted directed graph $G=(V, w)$ is strongly connected if and only if $\forall u, v \in V$, there exists a directed path from $u$ to $v$. (\textcolor{red}{This assumption needs to be discussed:} In our discussion of the learned weighted edge mask, we throw away edges $u \rightarrow v$ such that $w(u,v)$ and $w(v, u)$ are both \textcolor{red}{small}, and we keep edges $u \rightarrow v$ and $v \rightarrow u$ if at least $w(u,v)$ and $w(v, u)$ are considered \textcolor{red}{large enough}. In this case, the weighted directed graph is strongly connected, moreover if $u \rightarrow v$ then $v \rightarrow u$, only in the sense that one of the edge will have very small edge weight)
\end{definition}

\begin{definition}
\textcolor{red}{(Transition probability)} The \textit{transition probability kernel} $P: V \times V \rightarrow[0,1]$ is defined as $P(x, y):=\frac{w_{x y}}{w(x)}$, where $w(x):=\sum_{y \in V} w_{x y}$ as the normalizing constant for each node $x$.
\end{definition}

\begin{definition}\label{Perron measure}
\textcolor{red}{(Perron Measure)} Suppose $G=(V, w)$ is a finite and strongly connected weighted directed graph, then by Perron-Frobenius theorem, there exists a unique (up to scaling) positive function $m: V \rightarrow(0, \infty)$ such that $m(x)=\sum_{y \in V} m(y) P(y, x)$. Then a probability measure $\mathfrak{m}: V \rightarrow(0,1]$ on $V$ satisfying $\mathfrak{m}(x)=\sum_{y \in V} \mathfrak{m}(y) P(y, x)$ is called a \textit{Perron measure}. For a non-empty subset $\Omega \subset V$, its measure is defined as
$\mathfrak{m}(\Omega):=\sum_{x \in \Omega} \mathfrak{m}(x)$. 
\end{definition}

\begin{definition}\label{Inter Perron measure}
    Based on Perrson measure, we define a function $\mathfrak{m}: V \times V \rightarrow[0, \infty)$ by
    $$\mathfrak{m}(x, y):=\frac{1}{2}(\mathfrak{m}(x) P(x, y)+\mathfrak{m}(y) P(y, x))=\mathfrak{m}(x) \mathcal{P}(x, y),$$
    where we write $\mathfrak{m}(x, y)$ by $\mathfrak{m}_{x y}$. The following basic properties hold: 
    \begin{itemize}
        \item $\mathfrak{m}_{x y}=\mathfrak{m}_{y x}$
        \item $\mathfrak{m}_{x y}>0$ if and only if $y \in \mathcal{N}_x$ (or equivalently, $x \in N_y$ )
        \item $\mathcal{P}(x, y)=\mathfrak{m}_{x y} / \mathfrak{m}(x)$
    \end{itemize}
\end{definition}

\begin{definition}
\textcolor{red}{(mean transition probability)} Let $\mathfrak{m}$ be the Perron measure for $G=(V, w)$. We define \textit{reverse transition probability kernel} $\overleftarrow{P}: V \times V \rightarrow[0,1]$ by 
\begin{equation}
\overleftarrow{P}(x, y):=\frac{\mathfrak{m}(y)}{\mathfrak{m}(x)} P(y, x).
\end{equation}

and the \textit{mean transition probability kernel} $\mathcal{P}: V \times V \rightarrow[0,1]$ by 
\begin{equation}
\mathcal{P}:=\frac{1}{2}(P+\overleftarrow{P}). \label{mean transition kernel}
\end{equation}
\end{definition}

\textbf{Remark} It is worth noticing that for fixed node $x$, $\mathcal{P}(x, y)$ is a probability measure on the out-vertices of $x$. Namely, $\sum_{y \in V} \mathcal{P}(x, y) = 1$. And $\forall y \in V$, if $x \not \to y$, $\mathcal{P}(x, y) = 0$.

\textbf{Remark} In addition, when $G = (V, E)$ is an unweighted undirected graph, the positive function $m(x)$ specified in the Perron-Frobenius theorem is proportional to the inverse degree $\frac{1}{\deg(x)}$ at each node x, which is straightforward by considering an eigen-decomposition of the transition kernel. Therefore, the mean transition probability $\mathcal{P}(x, y)$ for $G$ is $\deg(x)$ if and only if $x$ is connected to $y$, which coincides with the transition kernels used in \textcolor{red}{(citations)}.

\begin{definition}
\textcolor{red}{(Notations in optimal transport theory)} Let $(V, w)$ denote a strongly connected, finite weighted directed graph. For two probability measures $\nu_0, \nu_1$ on $V$, a probability measure $\pi: V \times V \rightarrow[0, \infty)$ is called a coupling of $\left(\nu_0, \nu_1\right)$ if
$$
\sum_{y \in V} \pi(x, y)=\nu_0(x), \quad \sum_{x \in V} \pi(x, y)=\nu_1(y).
$$
Let $\Pi\left(\nu_0, \nu_1\right)$ denote the set of all couplings of $\left(\nu_0, \nu_1\right)$. The $\left(L^1-\right)$ Wasserstein distance from $\nu_0$ to $\nu_1$ is defined as
\begin{equation}
W\left(\nu_0, \nu_1\right):=\inf _{\pi \in \Pi\left(\nu_0, \nu_1\right)} \sum_{x, y \in V} d(x, y) \pi(x, y). \label{l1 distance}
\end{equation}
\end{definition}

\begin{definition}
For $\varepsilon \in[0,1]$ and $x \in V$, we define a probability measure $\nu_x^{\varepsilon}: V \rightarrow[0,1]$ by
\begin{equation}
\nu_x^{\varepsilon}(z):= \begin{cases}\varepsilon & \text { if } z=x \\ (1-\varepsilon) \mathcal{P}(x, z) & \text { if } z \neq x\end{cases},
\end{equation}
where $\mathcal{P}$ is the mean transition kernel we defined in \ref{mean transition kernel}
\end{definition}

Now we are equipped with enough mathematical tools to define ricci curvature for strongly connected weighted directed graphs.

\begin{definition}
For $x, y \in V$ with $x \neq y$, we define $\epsilon-$\textit{ricci curvature} by
\begin{equation}
\kappa_{\varepsilon}(x, y):=1-\frac{W\left(\nu_x^{\varepsilon}, \nu_y^{\varepsilon}\right)}{d(x, y)}
\end{equation}
where we use the Wasserstein distance defined in \ref{l1 distance}. Then we define the \textit{ricci curvature} on strongly connected weighted directed graphs by

\begin{equation}
\kappa(x, y):=\lim _{\varepsilon \rightarrow 1} \frac{\kappa_{\varepsilon}(x, y)}{1 - \varepsilon}
\end{equation}
\end{definition}

\begin{theorem}\label{without 4-cycles}
On a weighted directed locally finite graph $G$=$(V, w)$, where $\forall x, y \in V$, if $x \to y$ then $y \to x$, we have that if $x$ is connected to $y$ then

$\begin{aligned} \kappa(x, y) \geq & -\left(1-\mathcal{P}(x, y)-\mathcal{P}(y, x)-\sum_{x_1, x_1 \sim x, x_1 \sim y} \mathcal{P}(x, x_1) \vee \mathcal{P}(y, x_1)\right)_{+} \\ & -\left(1-\mathcal{P}(x, y)-\mathcal{P}(y, x)-\sum_{x_1, x_1 \sim x, x_1 \sim y} \mathcal{P}(x, x_1) \wedge \mathcal{P}(y, x_1)\right)_{+}+\sum_{x_1, x_1 \sim x, x_1 \sim y} \mathcal{P}(x, x_1) \wedge \mathcal{P}(y, x_1) ,\end{aligned}$

where $\mathcal{P}(x,y)$ corresponds to the mean transition probability from $x \to y$ defined in \ref{mean transition kernel}, $a \vee b := \max \{a, b\}$ and $a \wedge b := \min \{a, b\}$.
\end{theorem}

\textbf{Remark} \textcolor{red}{(Potential edge removal)} When dealing with the \textcolor{red}{mask}, we remove directed edges with weights under a certain threshold. But we need the directed graph to be strongly connected, otherwise the graph loses good spectral properties which hinders us to relate curvature to bottleneck on the graph. Therefore, to ensure a strongly connected directed graph, in the trimming process, we keep both $(u, v)$ and $(v, u)$ when at least one of $w(u, v)$ and $w(v, u)$ is relatively large. 

\textbf{Remark} For unweighted-undirected graphs, we have the following lower bound:

$\begin{aligned} \kappa(x, y) \geq & -\left(1-\frac{1}{\deg(x)}-\frac{1}{\deg(y)}-\frac{\# \Delta}{\deg(x) \wedge \deg(y)}\right)_{+} \\ & -\left(1-\frac{1}{\deg(x)}-\frac{1}{\deg(y)}-\frac{\# \Delta}{\deg(x) \vee \deg(y)}\right)_{+}+\frac{\# \Delta}{\deg(x) \vee \deg(y)} ,\end{aligned}$

 where $\# \Delta$ := number of common neighbors of node $x$ and $y$. In particular, the term $\sum_{x_1, x_1 \sim x, x_1 \sim y} \mathcal{P}(x, x_1) \wedge \mathcal{P}(y, x_1)$ is an extension of $\frac{\# \Delta}{\deg(x) \vee \deg(y)}$ with weighted edges, which we will see shortly in the proof.

Firstly, we define the following terms which will come up frequently in the proof:

\begin{enumerate}
    \item $\overrightarrow{N}_x:=\{y \in V \mid x \rightarrow y\}, \overleftarrow{N}_x:=\{y \in V \mid y \rightarrow x\}, N_x:=\overrightarrow{N}_x \cup \overleftarrow{N}_x$, which are \textit{inner neighborhood}, \textit{outer neighborhood} and \textit{neighborhood} respectively. If $\forall i, j \in V$, $i \to j$ implies $j \to i$, then $\overrightarrow{N}_x = \overleftarrow{N}_x = N_x$. Hence we use notation $N_x$ as neighborhood for convenience.
    \item ${\Delta}(x, y):=N_x \cap N_y$, the number of triangles based at the edge $x \sim y$. 
    \item $E(x, y):=$ $\sum_{x_1, x_1 \sim x, x_1 \sim y} (\mathcal{P}(x, x_1) -\mathcal{P}(y, y_1))_+ = \sum_{x_1 \in {\Delta}(x, y)} (\mathcal{P}(x, x_1) -\mathcal{P}(y, y_1))_+$, which is the excessive mass within the common neighbors of $x, y$ that needs to be transported out.
    \item $R(x, y):=$ $\sum_{x_1, x_1 \sim x, x_1 \sim y} (\mathcal{P}(y, x_1) -\mathcal{P}(x, y_1))_+ = \sum_{x_1 \in {\Delta}(x, y)} (\mathcal{P}(y, x_1) -\mathcal{P}(x, y_1))_+$, which is the remaining mass within the common neighbors of $x, y$ that needs to be filled up.
    \item $\mathcal{Q}(x|y)$:= $\{u \in V \mid u \sim x \text { and } u \not \sim y\}$, denotes the neighbors of x that are not connected to y.
    \item $A:= 1-\mathcal{P}(x, y)-\mathcal{P}(y, x)-\sum_{x_1, x_1 \sim x, x_1 \sim y} \mathcal{P}(x, x_1) \vee \mathcal{P}(y, x_1)$ and $B:= 1-\mathcal{P}(x, y)-\mathcal{P}(y, x)-\sum_{x_1, x_1 \sim x, x_1 \sim y} \mathcal{P}(x, x_1) \wedge \mathcal{P}(y, x_1)$
\end{enumerate}

\begin{proof}
We divide the proof into three different cases according to the size of $A$ and $B$. In each case, we resort to find a sub-optimal transportation plan providing an upper bound for $W\left(\nu_x^{\varepsilon}, \nu_y^{\varepsilon}\right)$ hence a lower bound for $\kappa(x, y)$.

When $0 \leq A \leq B$, we consider the following two sets of moves:

\begin{itemize}
    \item Move the initial mass $\mathcal{P}(x, y)$ on node $y$ to $\mathcal{Q}(y|x)$, then move $E(x, y)$ mass from $\Delta(x, y)$ to $\mathcal{Q}(y|x)$.
    \item Move $\mathcal{P}(x, y)$ mass from $\mathcal{Q}(x|y)$ to node $x$, then move $R(x, y)$ mass from $\mathcal{Q}(x|y)$ to $\Delta(x, y)$.
\end{itemize}

The first set of moves is feasible if and only if the following condition holds:
$$
1 - \mathcal{P}(y, x) - \sum_{x_1 \in \Delta(x, y)} \mathcal{P}(y, x1) \geq E(x, y) + \mathcal{P}(x, y)
$$
which is equivalent to
$$
$$

Therefore, 
\begin{align*}
&1 - \mathcal{P}(y, x) - \sum_{x_1 \in \Delta(x, y)} \mathcal{P}(y, x1) - E(x, y) - \mathcal{P}(x, y) \geq 0 \\
\iff &1 - \mathcal{P}(y, x) - \mathcal{P}(x, y) - \sum_{x_1 \in \Delta(x, y)} ((\mathcal{P}(x, x1) - \mathcal{P}(y, x1))_{+} + \mathcal{P}(y, x1)) \geq 0 \\
\iff &1 - \mathcal{P}(y, x) - \mathcal{P}(x, y) - \sum_{x_1 \in \Delta(x, y)} \mathcal{P}(x, x1) \vee \mathcal{P}(y, x1) \geq 0\\
\iff &A \geq 0 
\end{align*}

Hence $A \geq 0$ guarantees the first set of moves.

The condition for the second set of moves to hold is:
$$
1 - \mathcal{P}(x, y) - \sum_{x_1 \in \Delta(x, y)} \mathcal{P}(x, x1) \geq R(x, y) + \mathcal{P}(y, x)
$$
Similarly we get the equivalent condition:
$$
1 - \mathcal{P}(x, y) - \mathcal{P}(y, x) - \sum_{x_1 \in \Delta(x, y)} ((\mathcal{P}(y, x1) - \mathcal{P}(x, x1))_{+} + \mathcal{P}(x, x1))
$$
which is also guaranteed by $A \geq 0$.

Therefore we propose the following transportation plan:

\begin{enumerate}
    \item Move the initial mass $\mathcal{P}(x, y)$ on node $y$ to $\mathcal{Q}(y|x)$ with distance $1$.
    \item Move $E(x, y)$ mass from $\Delta(x, y)$ to $\mathcal{Q}(y|x)$ with distance at most $2$.
    \item Move $\mathcal{P}(x, y)$ mass from $\mathcal{Q}(x|y)$ to node $x$ with distance $1$.
    \item Move $R(x, y)$ mass from $\mathcal{Q}(x|y)$ to $\Delta(x, y)$ with distance at most $2$.
    \item Move the remaining mass in $\mathcal{Q}(x|y)$ to $\mathcal{Q}(x|y)$ to balance, with distance at most $3$.
    \item Move mass $\epsilon$ from node $x$ to node $y$
\end{enumerate}

By summing up all the costs we find:
\begin{align*}
W\left(\nu_x^{\varepsilon}, \nu_y^{\varepsilon}\right) &\leq (1-\epsilon)\{\mathcal{P}(x, y) + 2 \sum_{x_1 \in \Delta(x, y)} ((\mathcal{P}(x, x_1) - \mathcal{P}(y, x_1))_{+} + \mathcal{P}(y, x) + 2 \sum_{x_1 \in \Delta(x, y)} ((\mathcal{P}(y, x1) - \mathcal{P}(x, x_1))_{+} \\
&+ 3(1 - \mathcal{P}(x, y) - \mathcal{P}(y, x) - \sum_{x_1 \in \Delta(x, y)} \mathcal{P}(x, x_1) - \sum_{x_1 \in \Delta(x, y)} (\mathcal{P}(y, x_1) - \mathcal{P}(x, x_1))_{+})\} + \epsilon
\end{align*}

Therefore,
\begin{align*}
\kappa_{\varepsilon}(x, y) &\geq -(1-\epsilon)\{\mathcal{P}(x, y) + 2 \sum_{x_1 \in \Delta(x, y)} ((\mathcal{P}(x, x_1) - \mathcal{P}(y, x_1))_{+} + \mathcal{P}(y, x) + 2 \sum_{x_1 \in \Delta(x, y)} ((\mathcal{P}(y, x_1) - \mathcal{P}(x, x_1))_{+} \\
&+ 3(1 - \mathcal{P}(x, y) - \mathcal{P}(y, x) - \sum_{x_1 \in \Delta(x, y)} \mathcal{P}(x, x_1) - \sum_{x_1 \in \Delta(x, y)} (\mathcal{P}(y, x_1) - \mathcal{P}(x, x_1))_{+})\} + (1 - \epsilon) \\
&= (1 - \epsilon)(-3 + 2 \mathcal{P}(x, y) + 2 \mathcal{P}(y, x) + \sum_{x_1 \in \Delta(x,y)} \mathcal{P}(x, x_1) \vee \mathcal{P}(y, x_1) + 2 \sum_{x_1 \in \Delta(x, y)} \mathcal{P}(x, x_1) \wedge \mathcal{P}(y, x_1)) \\
&+ (1 - \epsilon) 
\end{align*}

Hence,
\begin{align*}
\kappa(x, y)&:=\lim _{\varepsilon \rightarrow 1} \frac{\kappa_{\varepsilon}(x, y)}{1 - \varepsilon}\\
&\geq -3 + 2 \mathcal{P}(x, y) + 2 \mathcal{P}(y, x) + \sum_{x_1 \in \Delta(x,y)} \mathcal{P}(x, x_1) \vee \mathcal{P}(y, x_1) + 2 \sum_{x_1 \in \Delta(x, y)} \mathcal{P}(x, x1) \wedge \mathcal{P}(y, x_1) + 1 \\
&= -2 + 2 \mathcal{P}(x, y) + 2 \mathcal{P}(y, x) + \sum_{x_1 \in \Delta(x,y)} \mathcal{P}(x, x_1) \vee \mathcal{P}(y, x_1) + 2 \sum_{x_1 \in \Delta(x, y)} \mathcal{P}(x, x_1) \wedge \mathcal{P}(y, x_1)
\end{align*}

When $A < 0 \leq B$, consider the following two sets of moves:

\begin{itemize}
    \item Move initial mass $\mathcal{P}(x, y)$ on y to fill remaining mass $\Delta(x, y)$ and $\mathcal{Q}(y|x)$.
    \item Move excessive mass in $\Delta(x, y)$ and mass in $\mathcal{Q}(x|y)$ to fill mass required at node $x$.
\end{itemize}

The first set of moves is feasible if and only if the following condition holds:
$$
\mathcal{P}(x, y) \leq \{1 - \mathcal{P}(y, x) - \sum_{x_1 \in \Delta(x, y)} \mathcal{P}(y, x_1)\} + \sum_{x_1 \in \Delta(x, y)} ((\mathcal{P}(y, x_1) - \mathcal{P}(x, x_1))_{+}
$$
which is equivalent to
\begin{align*}
&1 - \mathcal{P}(y, x) - \mathcal{P}(x, y) + \sum_{x_1 \in \Delta(x, y)} \{((\mathcal{P}(y, x_1) - \mathcal{P}(x, x_1))_{+}  - \mathcal{P}(y, x_1)\}\geq 0 \\
\iff &1 - \mathcal{P}(y, x) - \mathcal{P}(x, y) - \sum_{x_1 \in \Delta(x, y)} \mathcal{P}(y, x_1) \wedge \mathcal{P}(x, x_1) \geq 0 \\
\iff & B \geq 0
\end{align*}
Hence the first set of moves is feasible if and only if $B \geq 0$.

Similar condition for the second sets of moves to hold is:
$$
\mathcal{P}(y, x) \leq \{1 - \mathcal{P}(x, y) - \sum_{x_1 \in \Delta(x, y)} \mathcal{P}(x, x_1)\} + \sum_{x_1 \in \Delta(x, y)} ((\mathcal{P}(x, x_1) - \mathcal{P}(y, x_1))_{+}
$$
which also amounts to $B \geq 0$.

Therefore we propose the following transportation plan:
\begin{enumerate}
    \item Move initial mass $\mathcal{P}(x, y)$ on y to fill remaining mass $\Delta(x, y)$ and $\mathcal{Q}(y|x)$ with distance 1.
    \item Move excessive mass in $\Delta(x, y)$ and mass in $\mathcal{Q}(x|y)$ to fill mass required at node $x$ with distance 1.
    \item Balance the mass in $\mathcal{Q}(x|y)$ and excessive mass in $\Delta(x, y)$ with mass in $\mathcal{Q}(y|x)$ and remaining mass in $\Delta(x, y)$, with distance at most 2.
    \item Move mass $\epsilon$ from node $x$ to node $y$.
\end{enumerate}

Sum up all the costs we get:

\begin{align*}
W\left(\nu_x^{\varepsilon}, \nu_y^{\varepsilon}\right) &\leq (1-\epsilon)\{\mathcal{P}(x, y) + \mathcal{P}(y, x) \\
&+ 2(1 - \mathcal{P}(x, y) - \mathcal{P}(y, x) - \sum_{x_1 \in \Delta(x, y)} \mathcal{P}(y, x_1) + \sum_{x_1 \in \Delta(x, y)} (\mathcal{P}(y, x_1) - \mathcal{P}(x, x_1))_{+})\} + \epsilon
\end{align*}

Therefore, 
\begin{align*}
\kappa_{\varepsilon}(x, y) &\geq -(1-\epsilon)\{\mathcal{P}(x, y) + \mathcal{P}(y, x) \\
&+ 2(1 - \mathcal{P}(x, y) - \mathcal{P}(y, x) - \sum_{x_1 \in \Delta(x, y)} \mathcal{P}(y, x_1) + \sum_{x_1 \in \Delta(x, y)} (\mathcal{P}(y, x_1) - \mathcal{P}(x, x_1))_{+})\} + (1 - \epsilon) \\
&= -(1-\epsilon)(2 -\mathcal{P}(x, y) -\mathcal{P}(y, x)) - 2 \sum_{x_1 \in \Delta(x, y)} \mathcal{P}(x, x_1) \wedge \mathcal{P}(y, x_1)) + (1 - \epsilon)
\end{align*}

Hence, 
\begin{align*}
\kappa(x, y)&:=\lim _{\varepsilon \rightarrow 1} \frac{\kappa_{\varepsilon}(x, y)}{1 - \varepsilon}\\
&\geq \mathcal{P}(x, y) + \mathcal{P}(y, x) + 2 \sum_{x_1 \in \Delta(x, y)} \mathcal{P}(x, x_1) \wedge \mathcal{P}(y, x_1) - 2 + 1 \\
&=\mathcal{P}(x, y) + \mathcal{P}(y, x) + 2 \sum_{x_1 \in \Delta(x, y)} \mathcal{P}(x, x_1) \wedge \mathcal{P}(y, x_1) - 1
\end{align*}

When $A \leq B < 0$, we have the following transport plan:
\begin{enumerate}
    \item Move the initial mass on node $y$ to fill up the remaining mass $R(x, y)$ in $\Delta(x, y)$ and mass in $\mathcal{Q}(y|x)$, with distance $1$.
    \item Move the excessive mass $E(x, y)$ in $\Delta(x, y)$ and mass in $\mathcal{Q}(x|y)$ to node $x$, with distance $1$.
    \item Balance the mass between node $x$ and node $y$, with distance $1$.
\end{enumerate}

Summing up the costs we get:

\begin{align*}
W\left(\nu_x^{\varepsilon}, \nu_y^{\varepsilon}\right) &\leq (1-\epsilon)\{  \mathcal{P}(x, y) + (1 - \mathcal{P}(x, y) - \sum_{x_1 \in \Delta(x, y)} \mathcal{P}(x, x_1) + \sum_{x_1 \in \Delta(x, y)} (\mathcal{P}(x, x_1) - \mathcal{P}(y, x_1))_{+})) \} + \epsilon
\end{align*}
Similar to previous cases, we get that:
$$
\kappa(x, y) \geq \sum_{x_1 \in \Delta(x, y)} \mathcal{P}(x, y) \wedge \mathcal{P}(y, x)
$$
\end{proof}

\textbf{Remark} In the proof of theorem 1, we notice that in the first case, we move the remaining mass of $\mathcal{Q}(x|y)$ to $\mathcal{Q}(y|x)$ for distance 3 in the final step, which can be further improved if there exists edges between $\mathcal{Q}(x|y)$ to $\mathcal{Q}(y|x)$. In the next theorem, we will take that into account and further improve a lower bound for our ricci curvature with the help of 4-cycles.

\begin{definition}
Let $\square(x, y):=\left\{k \in N(x) \backslash N(y), k \neq y: \exists w \in\left(N(k) \cap N(y)\right) \backslash N(x)\right\}$ be the set of nodes $k \in N(x)$ forming a 4-cycle based at $x \sim y$ without diagonals inside.
\end{definition}

\begin{definition}
For any weighted directed locally finite graph $G$=$(V, w)$, where $\forall i, j \in V$, if $i \to j$ then $j \to i$, if $U \subset V$, then we set
$$\mathcal{D}(U):=\{\varphi: U \rightarrow V,|U|=|\varphi(U)|,(z, \varphi(z)) \in E, \forall z \in U\},$$
where $\forall \varphi \in \mathcal{D}(U)$, $\varphi$ is an injection.
\end{definition}

\begin{definition}
For any edge $x \sim y$ we let
$$\sharp_{\square}^{\mathfrak{m}}(x, y):=\max \left\{|U|: U \subseteq \square(x, y), \exists \varphi: U \rightarrow \square(y, x), \varphi \in \mathcal{D}(U)\right\}$$
From now on, we use $\varphi^{\mathfrak{m}}$ to denote one such optimal pairing between $\square(x, y)$ and $\square(y, x)$.
\end{definition}

\begin{theorem}\label{with 4-cycles}
On a weighted directed locally finite graph $G$=$(V, w)$, where $\forall x, y \in V$, if $x \to y$ then $y \to x$, we have that if $x$ is connected to $y$ then we have:

$\begin{aligned} \kappa(x, y) \geq & -\left(1-\mathcal{P}(x, y)-\mathcal{P}(y, x)-\sum_{x_1 \in \Delta(x, y)} \mathcal{P}(x, x_1) \vee \mathcal{P}(y, x_1) - \sum_{x_1 \in \square(x, y)} \mathcal{P}(x, x_1) \wedge \mathcal{P}(y, {\varphi}^{\mathfrak{m}}(x_1)) \right)_{+} \\ 
& -\left(1-\mathcal{P}(x, y)-\mathcal{P}(y, x)-\sum_{x_1 \in \Delta(x, y)} \mathcal{P}(x, x_1) \wedge \mathcal{P}(y, x_1) - \sum_{x_1 \in \square(x, y)} \mathcal{P}(x, x_1) \wedge \mathcal{P}(y, {\varphi}^{\mathfrak{m}}(x_1)) \right)_{+} \\
&+\sum_{x_1 \in \Delta(x, y)} \mathcal{P}(x, x_1) \wedge \mathcal{P}(y, x_1).
\end{aligned}$
\end{theorem}

\begin{proof}
The proof of theorem \ref{with 4-cycles} highly imitates the proof of theorem \ref{without 4-cycles}, which divides into $3$ cases. The only difference is that now we consider a transportation plan after sending a mass of $\sum_{x_1 \in \square(i, j)} \mathcal{P}(x, x_1) \wedge \mathcal{P}(y, {\varphi}^{\mathfrak{m}}(x_1))$ along a shortcut between $\mathcal{Q}(x|y)$ to $\mathcal{ Q}(y|x)$.

For illustration, we show the most complex case where 
$$1-\mathcal{P}(x, y)-\mathcal{P}(y, x)-\sum_{x_1 \in \Delta(x, y)} \mathcal{P}(x, x_1) \vee \mathcal{P}(y, x_1) - \sum_{x_1 \in \square(x, y)} \mathcal{P}(x, x_1) \wedge \mathcal{P}(y, {\varphi}^{\mathfrak{m}}(x_1)) \geq 0$$

Under this assumption, we use the following transportation plan:
\begin{enumerate}
    \item Move a total mass of $\sum_{x_1 \in \square(i, j)} \mathcal{P}(x, x_1) \wedge \mathcal{P}(y, {\varphi}^{\mathfrak{m}}(x_1))$ traversing a 4-cycle via $x_1 \to w$, where $x_1 \in \square(x, y)$, $w = \varphi^{\mathfrak{m}}(x_1)$.
    \item Move the remaining mass in $\mathcal{Q}(x|y)$ to fill up the required mass $(1 - \epsilon)\mathcal{P}(y, x)$ on node $x$ and remaining mass $R(x, y)$ in $\Delta(x, y)$.
    \item Move the excessive mass $E(x, y)$ in $\Delta(x, y)$ and initial mass on node $y$ to fill the mass in $\mathcal{Q}(y|x)$.
    \item Balance the mass in $\mathcal{Q}(x, y)$ with mass in $\mathcal{Q}(y, x)$.
    \item Move a mass of $\epsilon$ from node $x$ to node $y$.
\end{enumerate}

By summing up all the costs we find:
\begin{align*}
W\left(\nu_x^{\varepsilon}, \nu_y^{\varepsilon}\right) &\leq (1-\epsilon)\{\mathcal{P}(x, y) + 2 \sum_{x_1 \in \Delta(x, y)} ((\mathcal{P}(x, x_1) - \mathcal{P}(y, x_1))_{+} + \mathcal{P}(y, x) + 2 \sum_{x_1 \in \Delta(x, y)} ((\mathcal{P}(y, x1) - \mathcal{P}(x, x_1))_{+} \\
&+ 3[1 - \mathcal{P}(x, y) - \mathcal{P}(y, x) - \sum_{x_1 \in \Delta(x, y)} \mathcal{P}(x, x_1) - \sum_{x_1 \in \Delta(x, y)} (\mathcal{P}(y, x_1) - \mathcal{P}(x, x_1))_{+} \\
&- \sum_{x_1 \in \square(x, y)} \mathcal{P}(x, x_1) \wedge \mathcal{P}(y, {\varphi}^{\mathfrak{m}}(x_1))] + \sum_{x_1 \in \square(x, y)} \mathcal{P}(x, x_1) \wedge \mathcal{P}(y, {\varphi}^{\mathfrak{m}}(x_1))\} + \epsilon
\end{align*}

Therefore,
\begin{align*}
\kappa_{\varepsilon}(x, y) &\geq -(1-\epsilon)\{\mathcal{P}(x, y) + 2 \sum_{x_1 \in \Delta(x, y)} ((\mathcal{P}(x, x_1) - \mathcal{P}(y, x_1))_{+} + \mathcal{P}(y, x) + 2 \sum_{x_1 \in \Delta(x, y)} ((\mathcal{P}(y, x1) - \mathcal{P}(x, x_1))_{+} \\
&+ 3[1 - \mathcal{P}(x, y) - \mathcal{P}(y, x) - \sum_{x_1 \in \Delta(x, y)} \mathcal{P}(x, x_1) - \sum_{x_1 \in \Delta(x, y)} (\mathcal{P}(y, x_1) - \mathcal{P}(x, x_1))_{+} \\
&- \sum_{x_1 \in \square(x, y)} \mathcal{P}(x, x_1) \wedge \mathcal{P}(y, {\varphi}^{\mathfrak{m}}(x_1))] + \sum_{x_1 \in \square(x, y)} \mathcal{P}(x, x_1) \wedge \mathcal{P}(y, {\varphi}^{\mathfrak{m}}(x_1))\} + (1 - \epsilon) \\ 
&= (1 - \epsilon)\{-3 + 2 \mathcal{P}(x, y) + 2 \mathcal{P}(y, x) + \sum_{x_1 \in \Delta(x,y)} \mathcal{P}(x, x_1) \vee \mathcal{P}(y, x_1) + 2 \sum_{x_1 \in \Delta(x, y)} \mathcal{P}(x, x_1) \wedge \mathcal{P}(y, x_1) \\
&+2 \sum_{x_1 \in \square(x, y)} \mathcal{P}(x, x_1) \wedge \mathcal{P}(y, {\varphi}^{\mathfrak{m}}(x_1))\} + (1 - \epsilon) 
\end{align*}

Hence,
\begin{align*}
\kappa(x, y)&:=\lim _{\varepsilon \rightarrow 1} \frac{\kappa_{\varepsilon}(x, y)}{1 - \varepsilon}\\
&\geq -3 + 2 \mathcal{P}(x, y) + 2 \mathcal{P}(y, x) + \sum_{x_1 \in \Delta(x,y)} \mathcal{P}(x, x_1) \vee \mathcal{P}(y, x_1) + 2 \sum_{x_1 \in \Delta(x, y)} \mathcal{P}(x, x1) \wedge \mathcal{P}(y, x_1)\\
&+ 2 \sum_{x_1 \in \square(x, y)} \mathcal{P}(x, x_1) \wedge \mathcal{P}(y, {\varphi}^{\mathfrak{m}}(x_1)) + 1 \\
&= -2 + 2 \mathcal{P}(x, y) + 2 \mathcal{P}(y, x) + \sum_{x_1 \in \Delta(x,y)} \mathcal{P}(x, x_1) \vee \mathcal{P}(y, x_1) + 2 \sum_{x_1 \in \Delta(x, y)} \mathcal{P}(x, x_1) \wedge \mathcal{P}(y, x_1)\\
&+ 2 \sum_{x_1 \in \square(x, y)} \mathcal{P}(x, x_1) \wedge \mathcal{P}(y, {\varphi}^{\mathfrak{m}}(x_1))
\end{align*}
\end{proof}

\begin{definition}
For a weighted directed locally finite graph $G$=$(V, w)$, where $\forall x, y \in V$, if $x \to y$ then $y \to x$, we have that if $x$ is connected to $y$, we define a weighted version of \textit{Balanced Forman curvature} for $x \sim y$:

$\begin{aligned} \operatorname{Ric}^{\mathfrak{w}}(x, y):= & -\left(1-\mathcal{P}(x, y)-\mathcal{P}(y, x)-\sum_{x_1 \in \Delta(x, y)} \mathcal{P}(x, x_1) \vee \mathcal{P}(y, x_1) - \sum_{x_1 \in \square(x, y)} \mathcal{P}(x, x_1) \wedge \mathcal{P}(y, {\varphi}^{\mathfrak{m}}(x_1)) \right)_{+} \\ 
& -\left(1-\mathcal{P}(x, y)-\mathcal{P}(y, x)-\sum_{x_1 \in \Delta(x, y)} \mathcal{P}(x, x_1) \wedge \mathcal{P}(y, x_1) - \sum_{x_1 \in \square(i, j)} \mathcal{P}(x, x_1) \wedge \mathcal{P}(y, {\varphi}^{\mathfrak{m}}(x_1)) \right)_{+} \\
&+\sum_{x_1 \in \Delta(x, y)} \mathcal{P}(x, x_1) \wedge \mathcal{P}(y, x_1),
\end{aligned}$
where by theorem \ref{with 4-cycles}, $\kappa(x, y) \geq \operatorname{Ric}^{\mathfrak{w}}(x, y)$ for all $x \sim y$.
\end{definition}

\subsection{Spectral property of the weighted curvature}
In order to relate the weighted Balanced Forman curvature to geometric and spectral property of the graph, we state a cheeger-type inequality on strongly-connected weighted-directed Graph. When weighted Balanced Forman curvature is bounded below, the \textit{Dirichlet isoperimetric constant} is also bounded below by a positively correlated function of $\inf _{y \in V \backslash\{x\}} \kappa(x, y)$.

\begin{definition}
    The \textit{Chung Laplacian} $\mathcal{L}$ is defined as 
    $$\mathcal{L} f(x):=f(x)-\sum_{u \in V} \mathcal{P}(x, y) f(y)$$
    for a function $f: V \rightarrow \mathbb{R}$.
\end{definition}

\begin{definition}
    For $x \in V$, we define the \textit{asymptotic mean curvature} $\mathcal{H}_x$ around $x$ by $$\mathcal{H}_x:=\mathcal{L} \rho_x(x),$$
    where $\rho_x: V \rightarrow \mathbb{R}$ is the distance function from $x$ defined as $\rho_x(y):=d(x, y)$.
\end{definition}

\begin{definition}
    For $x \in V$, the inscribed radius $\operatorname{InRad}_x V$ of $V$ at $x$ is defined by $$\operatorname{InRad}_x V:=\sup _{y \in V} \rho_x(y).$$
\end{definition}

\begin{definition}
    For a non-empty $\Omega \subset V$, its boundary measure is defined as
    $$\mathfrak{m}(\partial \Omega):=\sum_{y \in \Omega} \sum_{z \in V \backslash \Omega} \mathfrak{m}_{y z},$$
    where $\mathfrak{m}_{y z}$ is defined in definition \ref{Inter Perron measure}. \\
\end{definition}

\begin{definition}
    The \textit{Dirichlet isoperimetric constant} on $\mathcal{V}$ in turn is defined by
    $$\mathcal{I}_{\mathcal{V}}^D:=\inf _{\Omega} \frac{\mathfrak{m}(\partial \Omega)}{\mathfrak{m}(\Omega)},$$
    where $\mathfrak{m}(\Omega)$ is the Perron measure on set $\Omega$ defined in definition \ref{Perron measure}, and the infimum is taken over all non-empty subsets $\Omega \subset \mathcal{V}$.
\end{definition}
\textbf{Remark} \textcolor{red}{(the wording of the description of $\mathcal{I}_{\mathcal{V}}^D$ needs refinement)}\textit{Dirichlet isoperimetric constant} is the counterpart of cheeger constant in a strongly-connected weighted directed graph, which is an indication of ``bottleneck'' in a graph. Namely, the larger the value of $\mathcal{I}_{\mathcal{V}}^D$, the less likely oversquashing and bottlenecking is to occur across inter-community edges for weighted-directed graph.

\begin{definition}
    For $x \in V$ and $R \geq 1$ we set $E_R(x):=\left\{y \in V \mid \rho_x(y) \geq R\right\}$.
\end{definition}

\begin{theorem}\label{weighted cheeger constant}
Let $x \in V$. For $K \in \mathbb{R}$ we assume $\inf _{y \in V \backslash\{x\}} \kappa(x, y) \geq K$. For $\Lambda \in$ $(-\infty,-1]$ we also assume $\mathcal{H}_x \geq \Lambda$. For $D>0$ we further assume $\operatorname{InRad}_x V \leq D$. Then for every $R \geq 1$ with $K R+\Lambda>0$, we have
$$
\mathcal{I}_{E_R(x)}^D \geq \frac{K R+\Lambda}{D}
$$
\end{theorem}

\begin{proof}
We state the lower bound $\frac{K R+\Lambda}{D}$ for $\mathcal{I}_{E_R(x)}^D$ which is positively related to $\inf _{y \in V \backslash\{x\}} \kappa(x, y)$. Detailed proof can be found in \textcolor{red}{(Ricci curvature on strongly connected component Proposition 9.6)}. 
\end{proof}

\textbf{Remark} By theorem \ref{with 4-cycles}, we have that ricci curvature $\kappa(x, y) \geq \operatorname{Ric}^{\mathfrak{w}}(x, y)$ for all $x \sim y$. Combined with theorem \ref{weighted cheeger constant}, we could control the value of $\mathcal{I}_{E_R(x)}^D \geq \frac{K R+\Lambda}{D}$ if $\operatorname{Ric}^{\mathfrak{w}}(x, y)$ is bounded below by some constant $\mathcal{K}$. Therefore our weighted version of Balanced Forman curvature $\operatorname{Ric}^{\mathfrak{w}}(x, y)$, similar to the Balanced Forman curvature defined in \textcolor{red}{Graph curvature} for unweighted-undirected graph, provides strong theoretical tool to analyze bottlenecking and oversquashing for \textcolor{red}{a specific subset of weighted directed graphs}.

\begin{theorem} \textbf{Proof of Kantorovich duality theorem on asymetric distance function} \\
    \textbf{Kantorovich Proof outlines}
    \begin{enumerate}
        \item Lemma1: 1-Lipshitz function on a distance function that satisfies triangle inequality is C-convex
        \item Lemma2: Proving that the dual problem with a specific form
    \end{enumerate}

    \begin{enumerate}
        \item \textcolor{red}{Crucial connection between curvature and spectral property of weighted curvature}
        \item \textcolor{red}{Crucial result for calculating weighted curvature}

    \end{enumerate}
\end{theorem}

\begin{theorem} \textbf{Green's theorem on proving the cheeger-type inequality}
    \textcolor{red}{Green's theorem using shorted distance on weighted edges} 
\end{theorem}

\begin{theorem} \textbf{Properties of weighted-directed curvature}
    \begin{enumerate}
    \item \textcolor{red}{Weighted-directed curvature is bounded below, leading to the fact that the limit exists for any small $\varepsilon$, hence when $\varepsilon$ tends to $0$, weighted-directed curvature tends to the OR-curvature}
    \item \textcolor{red}{Consider a strongly-connected unweighted directed graph, the same kind of extension also holds}
    \item \textcolor{red}{The weighted-directed curvature is scale-free in the sense that scale all edge weights by a factor won't change curvatures}
    \end{enumerate}
\end{theorem}

\begin{theorem} \textbf{Curvature properties with Laplacian}
\end{theorem}

\begin{theorem} \textbf{Relation with cheeger type inequality that can be viewed as a measure of bottlenecking in the weighted-directed graphs}
\end{theorem}

\begin{theorem} \textbf{A lower that could be utilized to calculate weighted-directed curvature}
    \item \textcolor{red}{This can be used for tasks that require lower computational cost utilizing the weighted-directed curvature. But under the stronger condition that the weighted-directed graph is "undirected", but the weights on in and out edges can differ. Under this strong assumption, but very common real user case.}
\end{theorem}
